# Supplementary material for: Generating Situated Reflection Triggers about Alternative Solution Paths: A Case Study of Generative AI for Computer-Supported Collaborative Learning
Source: arXiv:2404.18262 source file (2024-04-28)
Supplement: Supplementary file 1 [file main.tex]

\section{Intervention Time Interval Analysis}
\label{sec:timing_appendix}
Here we present an analysis of expected spacing between interventions that we collected from past course data of the activity from an earlier iteration of the cloud computing course.
We did this analysis to determine the need for scheduling to ensure spacing between interventions (to ensure students have enough time to respond) and determined qualitatively that 300s or 5 minutes between interventions would give them ample time to respond.

For this analysis we simulated running our intervention algorithm over the historical SQL command logs from the previous iteration of the course and tagged the points where the interventions were fired.
Then we analyze the time elapsed between subsequent firings and analyzed their distribution as shown in figure~\ref{fig:time_interval_analysis}.
There are 10, 11 and 26 cases with less than 60s, 60-120s and 120-300s in between interventions, while for 98 (or 67.6\%) cases there is a gap of 5 or more minutes between interventions. 

We wanted to mitigate cases with less than a 300s gap, especially cases with a 1-2 minute gap as these wouldn't provide students with enough time to respond.
Therefore we came up with the intervention scheduling strategy described in section~\ref{sec:intervention_scheduling}

\begin{figure}[!ht]
    \centering
    \includegraphics[width=0.45\textwidth]{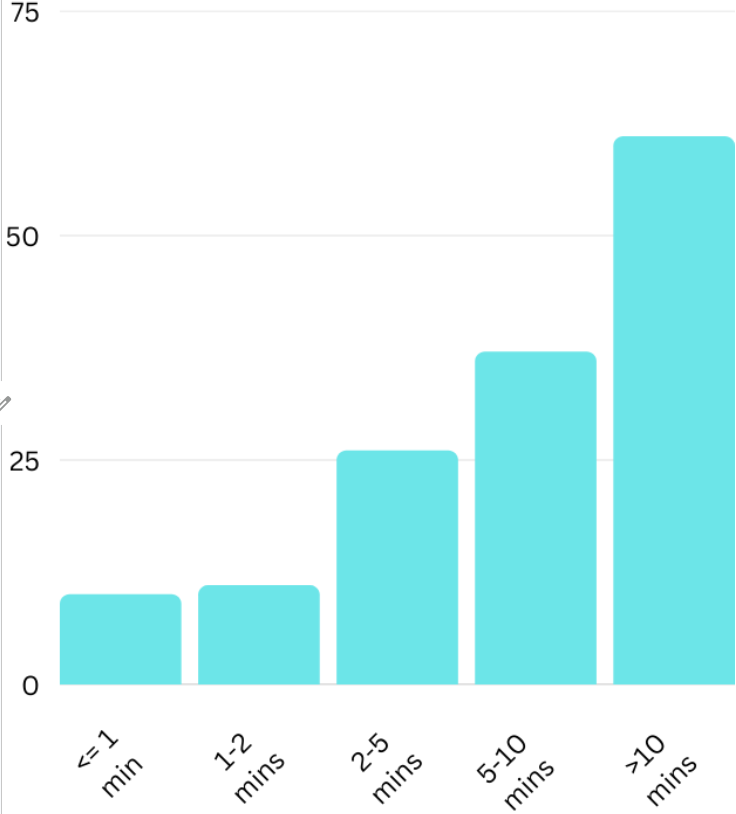}
    \caption{Distribution of time interval between consecutively triggered interventions for a simulated run of our intervention algorithm on past data of the activity.}
    \label{fig:time_interval_analysis}
\end{figure}

% Please add the following required packages to your document preamble:
% \usepackage{booktabs}
% \usepackage[normalem]{ulem}
% \useunder{\uline}{\ul}{}
\begin{table*}[!tbh]
\centering
\resizebox{\textwidth}{!}{%
\begin{tabular}{@{}ccll@{}}
\toprule
\textbf{SQL Command} &
  \textbf{Intervention} &
  \multicolumn{1}{c}{\textbf{Prompt to LLM}} &
  \multicolumn{1}{c}{\textbf{Output}} \\ \midrule
\begin{tabular}[c]{@{}c@{}}alter table result \\ modify salary INT\end{tabular} &
  DATATYPE\_COMPARISON &
   &
  \begin{tabular}[c]{@{}l@{}}Compare tradeoffs of using \\ VARCHAR vs INT\end{tabular} \\ \midrule
\begin{tabular}[c]{@{}c@{}}CREATE INDEX idx\_1 \\ ON result2 (dept\_name, title)\end{tabular} &
  \begin{tabular}[c]{@{}c@{}}COMPOSITE\_IND\_COL\_\\ ORDER\end{tabular} &
  \begin{tabular}[c]{@{}l@{}}Look at the following SQL table creation command:\\ CREATE TABLE result2 AS (SELECT employees.emp\_no, \\ employees.first\_name, employees.last\_name, \\ dept\_emp\_list.dept\_name, titles.title \\ FROM employees INNER JOIN dept\_emp\_list \\ ON employees.emp\_no=dept\_emp\_list.emp\_no \\ INNER JOIN titles \\ ON dept\_emp\_list.emp\_no=titles.emp\_no )\\ Now look at this command to create a composite index:\\ CREATE INDEX idx\_1 ON result2 (dept\_name, title)\\ Generate three plausible alternative composite \\ indices, including variants that switch the column \\ order from the original command. Just generate the \\ alternatives don't write any text or explanations:\end{tabular} &
  \begin{tabular}[c]{@{}l@{}}Consider the following alternative \\ composite indices:\\ CREATE INDEX idx\_2 \\ ON result2 (title, dept\_name);\\ CREATE INDEX idx\_3 \\ ON result2 (emp\_no, dept\_name);\\ CREATE INDEX idx\_4 \\ ON result2 (dept\_name, emp\_no);\\ Reflect on why the order of \\ columns matter in a composite index.\end{tabular} \\ \midrule
\begin{tabular}[c]{@{}c@{}}CREATE INDEX title\_index \\ ON task2(title)\end{tabular} &
  \begin{tabular}[c]{@{}c@{}}COMPOSITE\_VS\_MULTI\\ \_SINGLE\end{tabular} &
  \begin{tabular}[c]{@{}l@{}}Look at the following SQL table creation command:\\ CREATE TABLE task2 (SELECT e.*, d.dept\_no, \\ d.dept\_name, t.title, t.from\_date, t.to\_date \\ FROM employees AS e JOIN dept\_emp\_list AS d \\ ON e.emp\_no=d.emp\_no JOIN titles AS t \\ ON t.emp\_no=d.emp\_no)\\ Now look at this command to create a single column index:\\ CREATE INDEX title\_index ON task2(title)\\ Generate exactly one plausible composite index and \\ exactly one single column index for optimizing the \\ query. Just generate the alternatives don't write any \\ text or explanations:\end{tabular} &
  \begin{tabular}[c]{@{}l@{}}Consider the alternative composite index \\ and another single column index:\\ Composite index: CREATE INDEX \\ title\_dept\_index ON task2(title, dept\_name)\\ Single column index: CREATE INDEX \\ from\_date\_index ON task2(from\_date)\\ When should you choose a composite index \\ or multiple single column indices \\ for optimization?\end{tabular} \\ \midrule
\begin{tabular}[c]{@{}c@{}}SELECT e.first\_name, \\ e.last\_name, s.from\_date, \\ s.to\_date FROM salaries s \\ INNER JOIN employees e \\ ON s.emp\_no = e.emp\_no \\ WHERE s.salary \textgreater 100000\end{tabular} &
  \begin{tabular}[c]{@{}c@{}}DENORMALIZATION\_\\ WHEN\end{tabular} &
  \begin{tabular}[c]{@{}l@{}}Look at the following SQL queries \\ and useful denormalizations:\\ SQL Query: SELECT b.name, t.avg\_stars FROM \\ businesses b INNER JOIN (select business\_id, avg(stars) \\ avg\_stars FROM reviews GROUP BY business\_id) \\ t ON b.business\_id=t.business\_id  WHERE avg\_stars = 5;\\ Helpful Denormalization: CREATE TABLE \\ business\_star\_reviews AS (SELECT b.business\_id, b.name, \\ t.avg\_stars FROM businesses b INNER JOIN (SELECT \\ business\_id, avg(stars) avg\_stars FROM reviews GROUP \\ BY business\_id) t ON b.business\_id = t.business\_id);\\ SQL Query: SELECT e.first\_name, e.last\_name, \\ s.from\_date, s.to\_date FROM salaries s INNER JOIN \\ employees e ON s.emp\_no = e.emp\_no \\ WHERE s.salary \textgreater 100000\\ Helpful Denormalization:\end{tabular} &
  \begin{tabular}[c]{@{}l@{}}Consider this SQL command \\ for denormalization:\\ CREATE TABLE high\_earning\_employees \\ AS  (SELECT e.emp\_no, e.first\_name, \\ e.last\_name, s.from\_date, s.to\_date \\ FROM salaries s \\ INNER JOIN employees e\\ ON s.emp\_no = e.emp\_no\\ WHERE s.salary \textgreater 100000);\\ What are the trade-offs of using it?\end{tabular} \\ \midrule
\begin{tabular}[c]{@{}c@{}}CREATE TABLE emp\_title\_dept \\ AS (SELECT e.emp\_no, \\ e.first\_name, e.last\_name, t.title, \\ d.dept\_no FROM employees e \\ INNER JOIN dept\_emp\_list d \\ ON e.emp\_no = d.emp\_no \\ INNER JOIN titles t \\ ON d.emp\_no = t.emp\_no)\end{tabular} &
  \begin{tabular}[c]{@{}c@{}}TABLE\_CHOICE\_\\ DENORMALIZATION\end{tabular} &
  \begin{tabular}[c]{@{}l@{}}Given the SQL command to create a denormalized \\ table, generate alternatives that remove one of the \\ inner joins:\\ COMMAND: CREATE TABLE result2 AS \\ (SELECT employees.emp\_no, employees.first\_name, \\ employees.last\_name FROM employees \\ INNER JOIN dept\_emp\_list ON \\ employees.emp\_no=dept\_emp\_list.emp\_no INNER \\ JOIN titles ON dept\_emp\_list.emp\_no=titles.emp\_no)\\ \\ ALTERNATIVE: CREATE TABLE result2 AS \\ (SELECT employees.emp\_no, employees.first\_name, \\ employees.last\_name FROM employees INNER JOIN \\ dept\_emp\_list ON \\ employees.emp\_no=dept\_emp\_list.emp\_no)\\ \\ COMMAND: CREATE TABLE emp\_title\_dept AS \\ (SELECT e.emp\_no, e.first\_name, e.last\_name, t.title, \\ d.dept\_no FROM employees e INNER JOIN \\ dept\_emp\_list d ON e.emp\_no = d.emp\_no INNER JOIN \\ titles t ON d.emp\_no = t.emp\_no)\\ ALTERNATIVE:\end{tabular} &
  \begin{tabular}[c]{@{}l@{}}Consider this alternative denormalization:\\ CREATE TABLE emp\_title\_dept AS \\ (SELECT e.emp\_no, e.first\_name, \\ e.last\_name, t.title, d.dept\_no FROM \\ employees e INNER JOIN titles t \\ ON e.emp\_no = t.emp\_no)\\ Why would/wouldn't this be appropriate? \\ Think about the tradeoffs behind choosing \\ tables to join for denormalization.\end{tabular} \\ \bottomrule
\end{tabular}
}
\caption{Example LLM outputs for a given intervention triggered on a given SQL command along with the actual prompt given to the LLM (with relevant historical SQL context). The alternatives are syntactically correct.}
\label{tab:discussion_prompt_examples}
\end{table*}

\begin{figure*}[!tbh]
    \centering
    \includegraphics[width=0.8\textwidth]{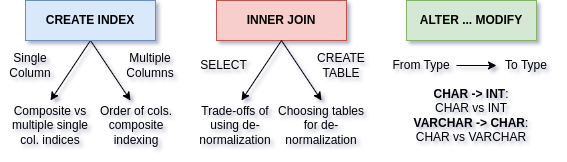}
    \caption{Overview of the intervention algorithm as a decision tree showing the intervention triggered and the SQL commands that trigger them.}
    \label{fig:activity_workflow}
\end{figure*}

\begin{figure*}[!tbh]
    \centering
    \includegraphics[width=\textwidth]{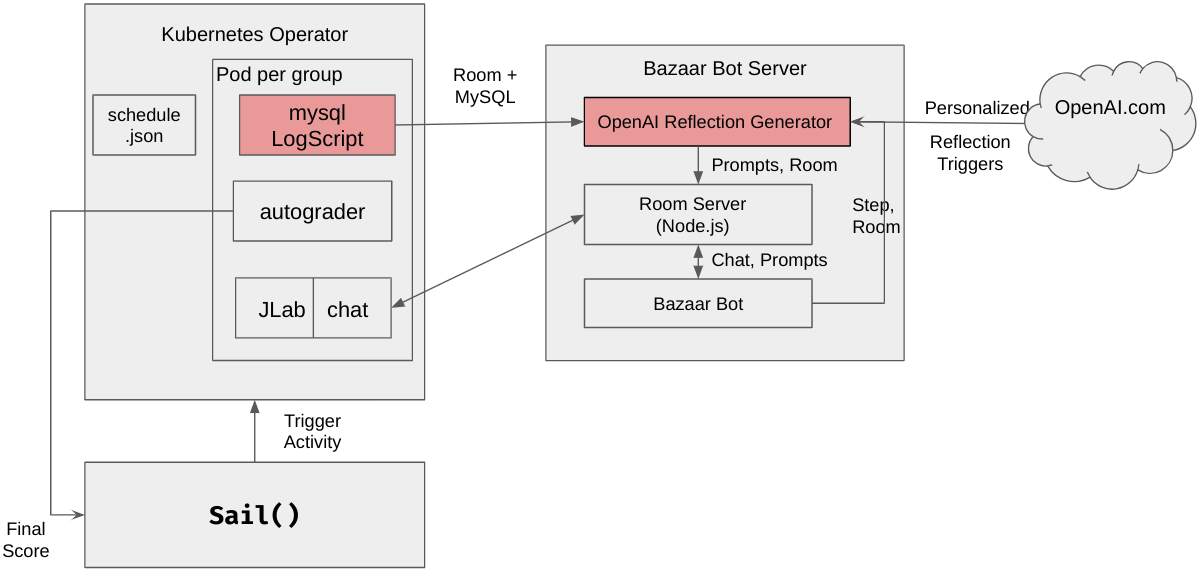}
    \caption{Overall system architecture of the computational environment of the activity. The ``MySQL'' hints refer to the ChatGPT-generated alternatives used for the discussion prompts.}
    \label{fig:activity_architecture}
\end{figure*}

\label{sec:appendix}
\section{Factorial Analysis}
\label{sec:factorial_analysis}
This section contains details about the factorial analysis. Figures~\ref{fig:fa1},~\ref{fig:fa2},~\ref{fig:fa3},~\ref{fig:fa4},~\ref{fig:fa5} show the residual component for each type of intervention.

\begin{figure*}[!ht]
    \centering
    \includegraphics[width=0.7\textwidth]{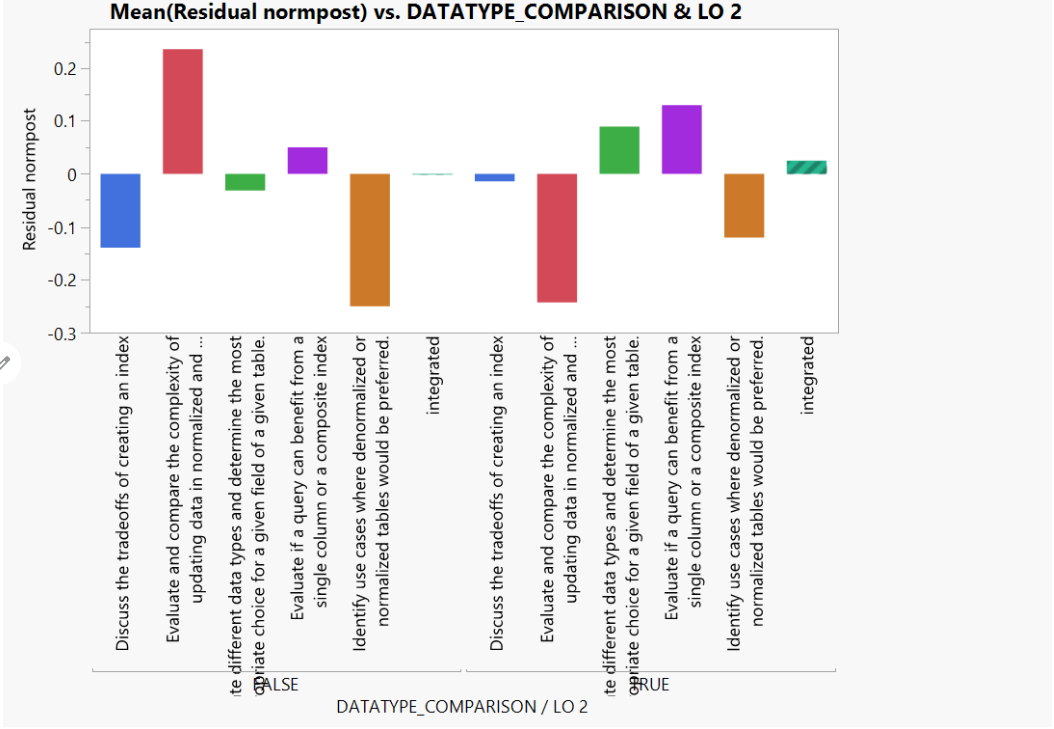}
    \caption{\textbf{Factorial Analysis:} residual component plot for the \texttt{DATATYPE\_COMPARISON} intervention}
    \label{fig:fa1}
\end{figure*}
\begin{figure*}[!ht]
    \centering
    \includegraphics[width=0.7\textwidth]{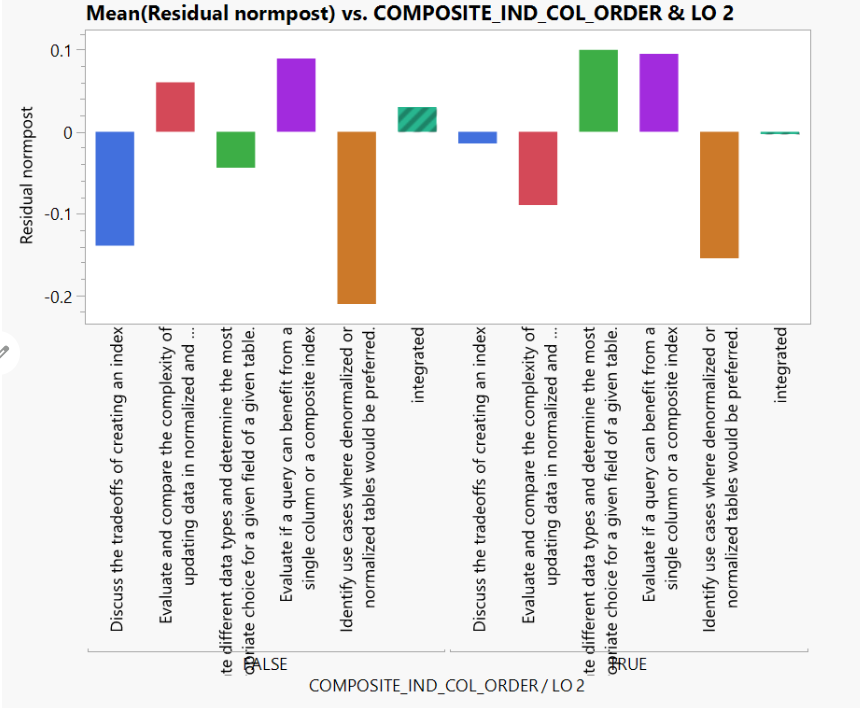}
    \caption{\textbf{Factorial Analysis:} residual component plot for the \texttt{COMPOSITE\_IND\_COL\_ORDER} intervention}
    \label{fig:fa2}
\end{figure*}
\begin{figure*}[!ht]
    \centering
    \includegraphics[width=0.7\textwidth]{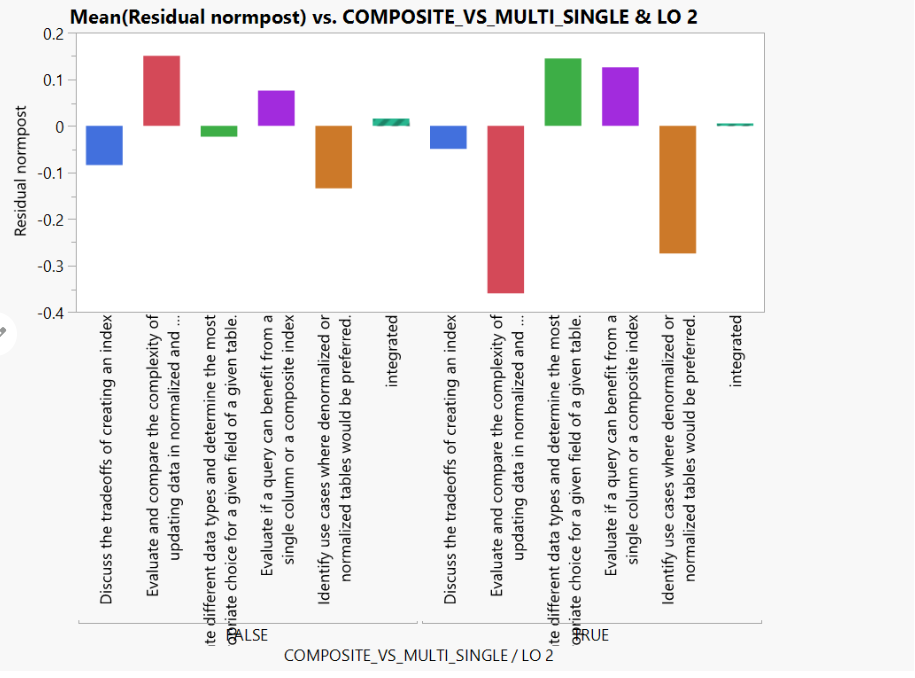}
    \caption{\textbf{Factorial Analysis:} residual component plot for the \texttt{COMPOSITE\_VS\_MULTI\_SINGLE} intervention}
    \label{fig:fa3}
\end{figure*}
\begin{figure*}[!ht]
    \centering
    \includegraphics[width=0.7\textwidth]{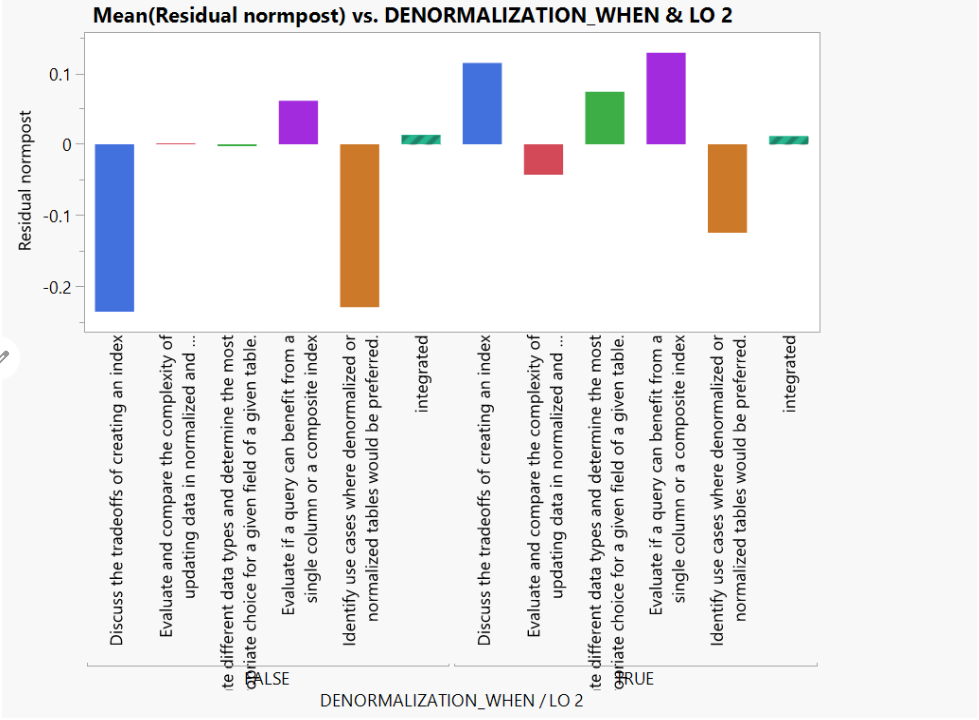}
    \caption{\textbf{Factorial Analysis:} residual component plot for the \texttt{DENORMALIZATION\_WHEN} intervention}
    \label{fig:fa4}
\end{figure*}
\begin{figure*}[!ht]
    \centering
    \includegraphics[width=0.7\textwidth]{pictures/COMPOSITE_VS_MULTI_SINGLE.png}
    \caption{\textbf{Factorial Analysis:} residual component plot for the \texttt{TABLE\_CHOICE\_DENORMALIZATION} intervention}
    \label{fig:fa5}
\end{figure*}

\begin{table}[!ht]
\centering
\resizebox{\textwidth}{!}{%
\begin{tabular}{@{}lll@{}}
\toprule
\multicolumn{1}{c}{\textbf{Intervention Type}} &
  \multicolumn{1}{c}{\textbf{Discussion Prompt}} &
  \multicolumn{1}{c}{\textbf{Student Response}} \\ \midrule
\texttt{COMPOSITE\_VS\_MULTI\_SINGLE} &
  \begin{tabular}[c]{@{}l@{}}"**DISCUSSION PROMPT:**\\ Consider the alternative composite index \\ and another single column index:\\ Single Column Index: CREATE INDEX \\ idx\_employees\_birthdate ON employees (birthdate);\\ Composite Index: CREATE INDEX \\ idx\_employees\_emp\_no\_birthdate ON employees (emp\_no, birthdate);\\ When should you choose a composite \\ index or multiple single column indices \\ for optimization?\end{tabular} &
  \begin{tabular}[c]{@{}l@{}}when searches have frequent multiple search conditions, \\ composite indices might help. But for queries such as \\ filtering on birthdate, the composite index on (emp\_no, \\ birthdate) will not have any benefit\end{tabular} \\ \midrule
\multirow{2}{*}{\texttt{DATATYPE\_COMPARISON}} &
  \multirow{2}{*}{\begin{tabular}[c]{@{}l@{}}"**DISCUSSION PROMPT:**\\ Compare tradeoffs of using \\ VARCHAR vs INT\end{tabular}} &
  \begin{tabular}[c]{@{}l@{}}INT is easier to search, requires less space, and \\ easier to index\end{tabular} \\ \cmidrule(l){3-3} 
 &
   &
  \begin{tabular}[c]{@{}l@{}}varchar is like string text which allows more \\ characters, while int is faster for comparison \\ and indexing\end{tabular} \\ \midrule
\texttt{COMPOSITE\_IND\_COL\_ORDER} &
  \begin{tabular}[c]{@{}l@{}}"**DISCUSSION PROMPT:**\\ Consider the following alternative \\ composite indices:\\ CREATE INDEX idx\_title\_emp\_no\_titles \\ ON titles(title, emp\_no)\\ CREATE INDEX idx\_emp\_no\_from\_date\_salary ...\\ Reflect on why the order of columns matter in a \\ composite index.\end{tabular} &
  I don't think we need date for task2 \\ \midrule
\multirow{2}{*}{\texttt{TABLE\_CHOICE\_DENORMALIZATION}} &
  \multirow{2}{*}{\begin{tabular}[c]{@{}l@{}}"**DISCUSSION PROMPT: PART (1/2)**\\ For this denormalization table creation command:\\ CREATE TABLE table2 AS (SELECT employees.emp\_no, \\ employees.first\_name, employees.last\_name...\\ \\ "**DISCUSSION PROMPT: PART (2/2)**\\ Consider this alternative denormalization:\\ CREATE TABLE table2 AS (SELECT employees.emp\_no... \\ Why would/wouldn't this be appropriate? Think about the \\ tradeoffs behind choosing tables to join for denormalization.\end{tabular}} &
  Because it is only joining two tables? \\ \cmidrule(l){3-3} 
 &
   &
  \begin{tabular}[c]{@{}l@{}}The 1st question, it only joins 2 tables, \\ still need a join on another table, \\ might be slower\end{tabular} \\
 &
   &
   \\ \bottomrule
\end{tabular}
}
\caption{}
\label{tab:student_responses}
\end{table}
